# Supplementary material for: Towards Next-Generation Urban Decision Support Systems through AI-Powered Construction of Scientific Ontology using Large Language Models -- A Case in Optimizing Intermodal Freight Transportation
Source: arXiv:2405.19255 source file (2024-09-06)
Supplement: Supplementary file 1 [file 70-appendix.tex]

\section{Appendix} \label{sec:Appendix}
